# Supplementary material for: Cuts in Graphs with Matroid Constraints
Source: arXiv:2406.19134 source file (2024-06-27)
Supplement: Supplementary file 1 [file appendix.tex]

\section{Appendix}

 \subsection{{\sf NP}-hardness of \dtai{2} when $G$ is Edgeless} \label{sec:genempty}
 
%\noindent{\bf Dilation $2$-Augmentation when $G$ is an empty graph(edgeless):} 

We prove that the \textsc{Dilation $2$-Augmentation} problem is \nph. when $G$ is an empty graph(edgeless).   Toward this we give a reduction from the {\sc $t$–Spanner} problem. Given a connected undirected unweighted graph $H$ and  a positive integers $k$, the {\sc $t$–Spanner} problem asks  to find a subset $E' \subseteq E(H)$ of size at most $k$ such that for each pair of vertices $u,v\in V(H)$ we have  $d_{H'}(u,v)\leq t\cdot d_{H}(u,v)$ where $H' = (V(H), E')$. The  {\sc $t$–Spanner} problem is known to be \nph even for $t=2$~\cite{PelegS89}.

% Let $(H,k)$ be any arbitrary instance of the $2$–Spanner Problem. 

Given an instance $(H,k)$ of {\sc $2$–Spanner} problem we construct an instance $(G,\Gamma, k')$ of \textsc{Dilation $2$-Augmentation} as follows. We set the graph $H$ as $\Gamma$. The graph $G$ is a subgraph of $\Gamma$ with $V(G)=V(\Gamma)$  and $E(G)=\emptyset$. This completes the description of the instance $(G,\Gamma,k')$ with $ k'=k$ (see Figure \ref{fig:edgeless} for an illustration of the construction).   It is easy to observe that this  construction can be done in time polynomial 
 in $V(H)$. Now we give the correctness of our reduction.

\begin{figure}[ht!]
	\centering
	\includegraphics[width=.8\textwidth]{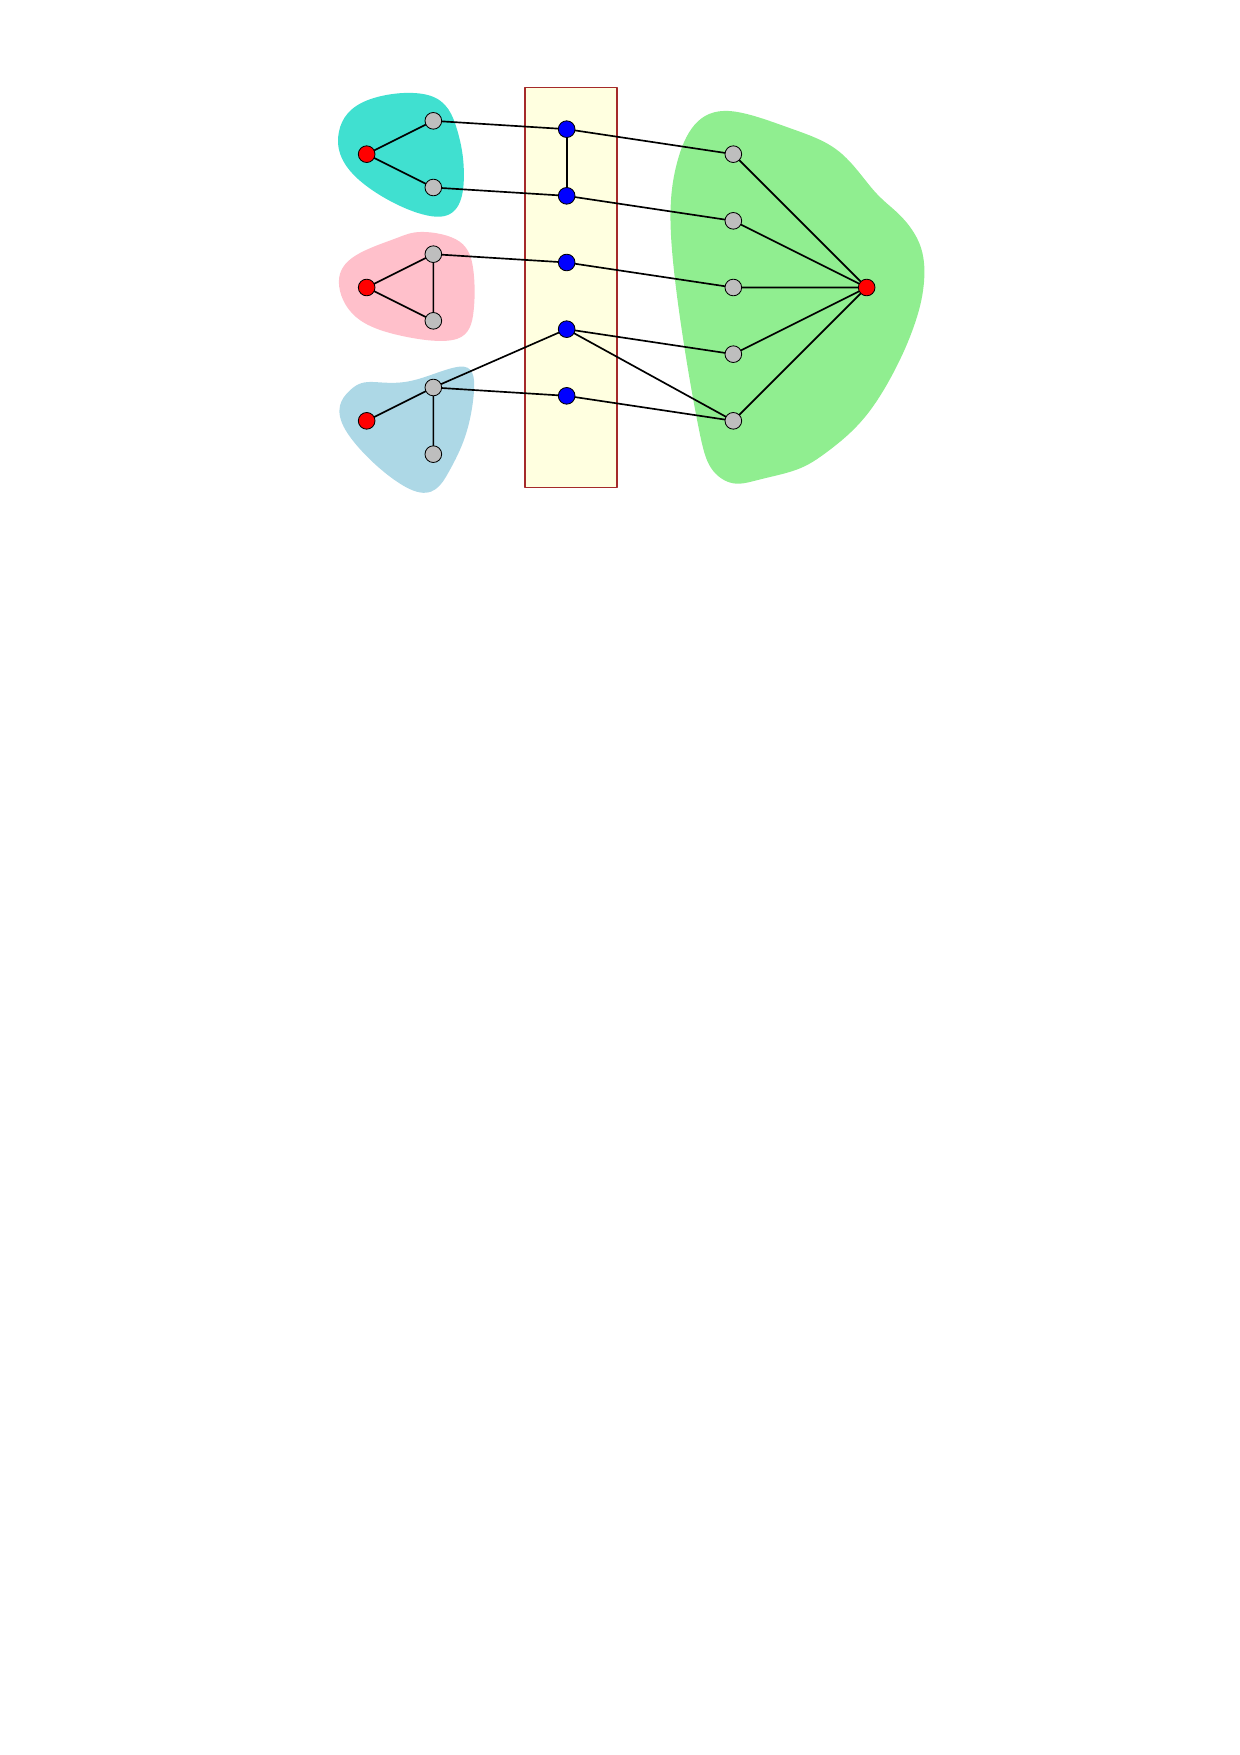}
	\caption{Hardness for $t=2$ when $G$ is an edgeless  graph.}
 \label{fig:edgeless}
\end{figure}

% \begin{itemize}
%     \item 
% \end{itemize}

% Consider the instance $(\mathcal{M},G)$ of \textsc{Dilation $2$-Augmentation} problem where $G$ is an empty (edgeless) graph on the set of vertices $V(H)$ and $\Gamma=H$. 

\begin{lemma}
  $(H,k)$ is a \yes-instance of {\sc $2$–Spanner} if and only if  $(G,\Gamma, k')$ is a \yes-instance of  \textsc{Dilation $2$-Augmentation}.
\end{lemma}

\begin{proof}
In the forward direction, let $(H,k)$ be a \yes-instance of \textsc{$2$–Spanner} problem and $S \subseteq E(H)$ be a solution. That means  for every pair of vertices in the graph $H'=(V(H), S)$ we have $d_{H'}(u,v)\leq 2\cdot d_{H}(u,v)$. Consider $S=T$. Now the graph $G+T$ is precisely $H'$. By definition, for each pair of vertices in $G$ we have $d_{G+T}(u,v)= d_{H'}(u,v) \leq 2\cdot d_{H}(u,v)= 2\cdot d_{\Gamma}(u,v)$. As $|T|=|S \leq k =k'$, $T$ is a solution for  \textsc{Dilation $2$-Augmentation} in the instance $(G,\Gamma, k')$.

In the backward direction, let $(G,\Gamma, k')$ be a \yes-instance of \textsc{Dilation $2$-Augmentation} problem and $T$ be a solution.  That means for every pair of vertices $u, v$ in $G$ we have $d_{G+T} (u,v) \leq 2 \cdot d_{\Gamma}(u,v)$. Further we assume that $T$ is minimal. Now we are in two cases.

\begin{description}
     \item[{Case (i)}: $T\subseteq E(\Gamma)$.] In this case,  $d_{H'}(u,v)\leq 2 \cdot  d_{\Gamma}(u,v)= 2 \cdot  d_{\Gamma}(u,v)$, where $H'= (V(H), T)$. So $T$ is a solution for the  \textsc{$2$–Spanner} problem on $(H,k)$.
     \medskip 
\item[{Case (ii)}: $T \setminus E(\Gamma) \neq \emptyset$.]
Let $e=(p,q)$ an edge in $T \setminus E(\Gamma)$. Consider any two vertices $u$ and $v$ that are adjacent in $\Gamma$. Observe that $d_{\Gamma}(u,v)=1$ so $d_{G+T}(u,v)\leq 2$. Now since $(p,q)\notin E(\Gamma)$ we have $d_{\Gamma}(p,q)\geq 2$. So  $d_{G+T}(p,q)\geq 2$. Thus between the vertices $p$ and $q$, there exists no shortest path of length at most two containing the edge $(p,q)$ in $G+T$. This contradicts the minimality of $T$. So this case can not appear.     
\end{description}
\end{proof}

Hence we have the following proposition.

\begin{proposition}\label{prop:empty}
    \textsc{Dilation $2$-Augmentation} is \nph~when $G$ is edgeless.
\end{proposition}

\subsection{{\sf W[2]}-hardness of \dtai{2} when  $\Gamma$ is  Clique} \label{sec:cliquegen}

Let $(G,\Gamma, k)$ be an instance of \dtwoa where $\Gamma$ is a complete graph, and $G$ is an arbitrary graph. Then, note that $d_{\Gamma}(u, v) = 1$ for all $u, v \in V(\Gamma)$, which implies that the weights of all the edges in $G$ is $1$, and the weight of any newly added edge is also $1$. In this case, \dtwoa is equivalent to deciding whether we can add $k$ new edges $S$ to $G$ such that the diameter of $G+S$ (i.e., maximum distance between any pair of vertices in $G+S$) is at most $2$. This corresponds to the well-known  {\sc Diameter Augmentation} problem which is known to be \wth~\cite{DBLP:journals/dam/GaoHN13}. Hence, we have the following proposition.

\begin{proposition}\label{prop:diamaug}
    \dtwoa is \wth~parameterized by $k$,  when $\Gamma$ is  clique.
\end{proposition}

% \vspace{5 pt}
% \section{Things to do}
%   \begin{itemize}
%         \item Notation same 
%         \item refer figures
%         \item check preliminaries
%         \item add conclusion
%         \item Organization of table and sections
%         \item Check all section, subsection name
%         \item Check Sloppy
%         \item any question mark
%         \item consistent of command: $\mathcal{O}, \yes, \no, \fpt, \woh$
%     \end{itemize}
